# Supplementary material for: Quantum Geometric Injection and Shift Optical Forces Drive Coherent Phonons
Source: arXiv:2507.17814 source file (2026-10-19)
Supplement: Supplementary file 1 [file suppmat.tex]

\documentclass[aps,onecolumn,superscriptaddress,notitlepage]{revtex4-1}

\bibliographystyle{apsrev4-1}

\usepackage{graphicx}
\usepackage{amsmath}
\usepackage{bm}
\usepackage{color}
\usepackage{comment}
\usepackage[percent]{overpic}
\usepackage[normalem]{ulem} 
\usepackage[bookmarks=true,colorlinks=true,urlcolor=blue,linkcolor=blue,citecolor=blue,breaklinks]{hyperref}

\usepackage{amssymb}
\usepackage{booktabs}

\usepackage{physics}

\usepackage[toc]{appendix}

%\usepackage{ulem}

  % Prefix figures with 'S'
\setcounter{figure}{0}  % Start figure counter from S1

  % Prefix equations with 'S'
\setcounter{equation}{0}  % Start equation counter from S1

\begin{document}

\sloppy

\newcommand{\blue}[1]{{\textcolor{blue} {#1}}}
\newcommand{\red}[1]{{\textcolor{red} {#1}}}
\newcommand{\green}[1]{{\textcolor{green} {#1}}}
%Title of paper
\title{Supplemental Material:\\ ``Quantum Geometric Injection and Shift Optical Forces Drive Coherent Phonons'' }

\author{J. Luke Pimlott}
\email{jlp62@bath.ac.uk}
\affiliation{Department of Physics, University of Bath, Claverton Down, Bath BA2 7AY, United Kingdom}

\author{Habib Rostami}
\email{hr745@bath.ac.uk}
\affiliation{Department of Physics, University of Bath, Claverton Down, Bath BA2 7AY, United Kingdom}

\maketitle

\tableofcontents

\section{Kadanoff-Baym Green's Function Approach to Deriving Raman Susceptibility} \label{app.KB_propagator}
In the presence of light–matter interaction with a light field with vector potential $\mathbf{A}$ and electron-phonon interaction operator $\hat{\cal M}_a$, phonon displacement field component $ u_a$, the thermodynamical average of the atomic force is expressed in terms of the field-dependent Green's function \cite{KadanoffBaym,Rostami2021,Rostami_prb_2021}
\begin{align}\label{eq:F}
    {\cal F}_a(1) = - i\int_{1'}\int_{1''} {\rm tr}[\hat {\cal M}_a(1',1'';1) \hat G(1'',1'^{+})] \eval_{\bf{u}\rightarrow0}.
\end{align}
Here, $1 = (\mathbf{r}_1, t_1)$ is a shorthand for the space-time coordinate, $1^{+}=(\mathbf{r}_1, t_1+0^+)$, ${\rm tr}[\dots]$ denotes the trace over internal spinor degrees of freedom, and the Green's function is defined as 
\begin{align}
    \hat G(1,1') = -i \langle {\cal T}_t[\hat\psi_{H}(1) \hat \psi^\dagger_{H}(1')] \rangle 
\end{align}
in which $\langle \cdots \rangle$ stands for the thermodynamical average, ${\cal T}_t$ denotes the time-ordering operation, and $\hat \psi_H(\mathbf{r}, t)$ is the field operator in the Heisenberg picture, expressed in the basis of the full Hamiltonian $\hat{\mathcal{H}}$, which includes kinetic, light–matter, and electron-phonon interaction terms. The electron-phonon coupling, $\hat {\cal M}_a$ reads 
\begin{align}
    \hat {\cal M}_a(1',1'';1) = - \frac{\delta \hat G^{-1}(1',1'')}{\delta u^a(1)}\Bigg|_{{\bf u}\to 0},
\end{align}
where the inverse Green's function obeys (note that $\hat{\mathcal{H}}(\mathbf{p})=\hat H({\mathbf p})+\hat M_a({\mathbf p}) u^a$ is the ${\mathbf p}$-resolved form of the Hamiltonian of Eq.~(1) in the main text)
\begin{align}
    \hat G^{-1}(1',1'') = \left\{i\partial_{t_{1'}} -\hat H(-i\hbar \nabla_{1'} + e{\bf A}(1')) - \hat M_a(-i\hbar \nabla_{1'} + e{\bf A}(1'))  u^a (1')\right\}\delta(1'-1''),
\end{align}
with $\hat H({\mathbf p}) \equiv\hat H(-i\hbar\nabla)$ the non-interacting electronic Hamiltonian, and the light-matter interaction included via minimal coupling, which can be Taylor expanded in small $\mathbf{A}$, giving paramagnetic (one-photon coupling) and diamagnetic (two-photon coupling) current operators, as 
\begin{align}
    \hat{H}({\bf p}) \rightarrow 
    \hat{H} ({\bf p} + e {\bf A}) \approx \hat{H}({\bf p}) + e [\nabla_{p_{b_1}} \hat{H}({\bf p})] A^{b_1} + \frac{e^2}{2} [\nabla_{p_{b_1}}\nabla_{p_{b_2}} \hat{H}({\bf p})] A^{b_1} A^{b_2} + \order{{\bf A}^3}. \label{eq:H-minimalcoupling}
\end{align}
Similarly, part of the light–matter coupling emerges as a mixed photon–phonon–electron interaction, originating from the (minimally-coupled) momentum dependence of the electron–phonon coupling, expanded to 
\begin{align}
    \hat{M}_a({\bf p}) \rightarrow 
    \hat{M}_a ({\bf p} + e {\bf A}) \approx \hat{M}_a({\bf p}) + e [\nabla_{p_{b_1}} \hat{M}_a ({\bf p})] A^{b_1} +  \frac{e^2}{2} [\nabla_{p_{b_1}} \nabla_{p_{b_2}} \hat{M}_a ({\bf p})] A^{b_1} A^{b_2} + \order{{\bf A}^3}, \label{eq:M-minimalcoupling}
\end{align}
with repeated indices summed according to the Einstein summation convention. Following the Taylor expansion, we define the one-photon and two-photon current operators, as well as photon-phonon-electron coupling terms in the space-time coordinate basis, based on the derivatives of the inverse Green's function,
\begin{align}
    &\nabla_{p_b}  \hat {H} 
    ~~~\to~~~ \hat j_b(1',1'';2) = \frac{\delta \hat G^{-1}(1',1'')}{\delta A^b(2)}
    \\
    &\nabla_{p_b} \nabla_{p_c} \hat {H}
    ~~~\to ~~~
    \hat j_{bc}(1',1'';2,3) = \frac{\delta^2 \hat G^{-1}(1',1'')}{\delta A^c(3) \delta A^b(2)}
    \\
    & \nabla_{p_b} \hat {M}_a
    ~~~\to~~~ \hat {\cal M}_{ab}(1',1'';1,2) = -\frac{\delta \hat G^{-1}(1',1'')}{\delta A^b(2) \delta u^{a}(1)}
    \\
    & \nabla_{p_b} \nabla_{p_c} \hat {M}_a
    ~~~\to~~~ \hat {\cal M}_{abc}(1',1'';1,2,3) = -\frac{\delta \hat G^{-1}(1',1'')}{\delta A^c(3) \delta A^b(2) \delta u^{a}(1)}
\end{align}
(noting that ${\delta G^{-1}}/{\delta A}=-{\delta \mathcal{H}}/{\delta A}$ and ${\delta G^{-1}}/{\delta u}=-{\delta\mathcal{H}}/{\delta u}$). With the light–matter coupling term expressed in terms of the Green's function, the Raman susceptibility can be obtained by applying a variational approach and differentiating Eq.~\eqref{eq:F} with respect to the light field:
\begin{align}
    \pi_{abc} (1;2,3) = \frac{1}{2} \frac{\delta^2 {\cal F}_a(1)}{\delta A_b(2)\delta A_c(3)} \Bigg|_{\bf A\to 0}.
\end{align}
The lengthy but straightforward variational 
calculus generates four distinct terms for the Raman response given by
\begin{align}
    \pi_{abc}(1;2,3) =  
    \frac{1}{2}(\pi^{\rm A}_{abc}(1;2,3) + \pi^{\rm B}_{abc}(1;2,3) + \pi^{\rm C}_{abc}(1;2,3) + \pi^{\rm D}_{abc}(1;2,3))
\end{align}
where each term explicitly reads 
\begin{align}
  \pi^{\rm A}_{abc}(1;2,3) &= - \int_{1',1''}   \int_{2',2''} \int_{3',3''} \bigg \{  \Tr[\hat{\cal M}_a(1',1'';1) G(1'',3') \hat{j}_c(3',3'';3) G(3'',2') \hat{j}_b(2',2'';2) G(2'',1')]  \nonumber \\
    &\hspace{3cm} + \Tr[\hat{\cal M}_a(1',1'';1) G(1'',2') \hat{j}_b(2',2'';2) G(2'',3') \hat{j}_c(3',3'';3) G(3'',1')] \bigg\}, \label{eq.pia}
\end{align}
\begin{align}
  \pi^{\rm B}_{abc}(1;2,3) &=  \int_{1',1''} \int_{2',2''} \bigg \{  \Tr[\hat{\cal M}_{ab}(1',1'';1,2) G(1'',2') \hat{j}_c(2',2'';3) G(2'',1')] + \nonumber \\
    &\hspace{2cm} + \Tr[\hat{\cal M}_{ac}(1',1'';1,3) G(1'',2') \hat{j}_b(2',2'';2) G(2'',1')] \bigg \}, \label{eq.pib}
\end{align}
\begin{align}
    \pi^{\rm C}_{abc}(1;2,3) =  \int_{1',1''} \int_{2',2''} \Tr[\hat{\cal M}_a(1',1'';1) G(1'',2') \hat{j}_{bc}(2',2'';2,3) G(2'',1')], \label{eq.pic}
\end{align}
and finally 
\begin{align}
     \pi^{\rm D}_{abc}(1;2,3) =- \int_{1',1''}  \Tr[\hat{\cal M}_{abc}(1',1'';1,2,3) G(1'',1')].  \label{eq.pid}
\end{align}
These terms can be illustrated using four distinct Feynman diagrams depicted in Fig. \ref{fig:feyn}. Finally, the gauge-invariant response function to the external electric fields, $\chi_{abc}$, is obtained by relating the electric field to a homogeneous vector potential, ${\bf E}(t) = -\partial_t {\bf A}(t)$, which in the frequency domain becomes ${\bf A}(\omega) = {\bf E}(\omega) / (i\omega)$, leading to 
\begin{align}
    \chi_{abc}(\omega_p;\omega_1,\omega_2) = \frac{\pi_{abc}(\omega_p;\omega_1,\omega_2)}{(i\omega_1)(i\omega_2)},
\end{align}
having Fourier transformed the susceptibility to the frequency domain, where our electric fields are $E^b(\omega_1)$ and $E^c(\omega_2)$, and with $\omega_p=\omega_1+\omega_2$ the frequency of the Raman force generated. Note that experimentally, one would observe both $\chi_{abc}(\omega_p;\omega_1,\omega_2)$ and $\chi_{acb}(\omega_p;\omega_2,\omega_1)$ simultaneously, which as they are equal means that the total observed response would be twice that implied by a single susceptibility component.
\begin{figure}
    \centering
    \begin{overpic}[width=\linewidth]{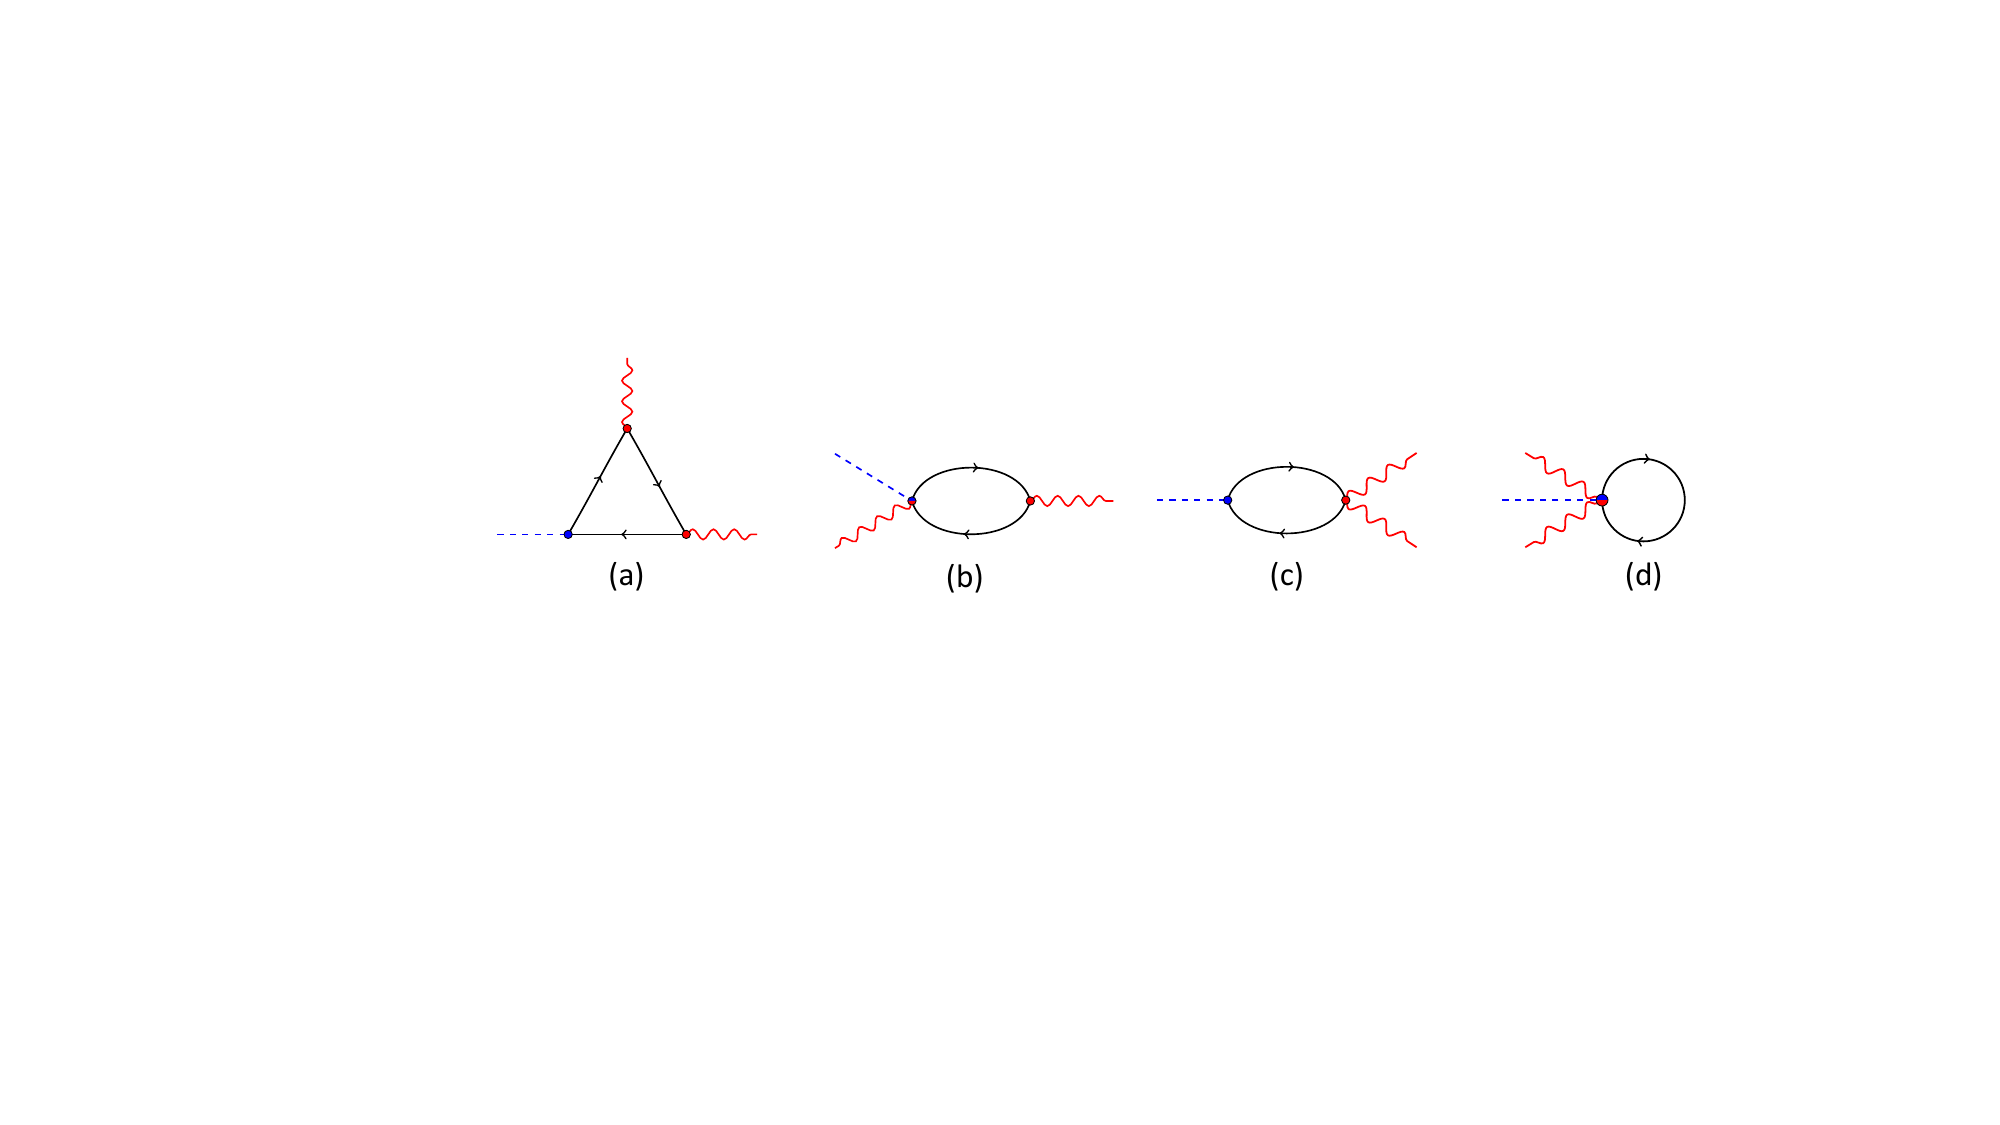}
        \put(10,-2){\large (a)}
        \put(38.5,-2){\large (b)}
        \put(65.5,-2){\large (c)}
        \put(95,-2){\large (d)}
    \end{overpic}
    \vspace{1mm}
    \caption{The four topologically-unique Feynman diagrams for the Raman force susceptibility: solid, dashed, and wavy lines respectively denote electrons, phonons, and photons. The diagrams from (a)–(d) respectively represent Eqs.~\eqref{eq.pia}–\eqref{eq.pid}. Diagrams (a) and (b) have two permutations.}
    \label{fig:feyn}
\end{figure}

\section{Formal expression of each diagram in the band basis} 
We use a Matsubara summation approach in the band basis to formally evaluate each diagram in terms of electronic dispersion, and the matrix elements of light-matter and electron-phonon coupling terms. First, we fix the notation as
\begin{align}
    \hat{j}_{b_1 b_2 \dots b_n} &= -e^n \hat{v}_{b_1 b_2 \dots b_n}, 
    & 
    \hat{\mathcal{M}}_{a b_1 b_2 \dots b_n} &= e^n \hat{M}_{a b_1 b_2 \dots b_n},
    \label{eq:nphotonvertex}
\end{align}
where $\hat{v}_b = \partial_{p_b} \hat{\mathcal{H}}$ is the velocity operator, 
$\hat{M}_a = \partial_{u_a} \hat{\mathcal{H}}$ is the electron-phonon coupling operator, and 
$\hat{M}_{ab} = \partial_{p_b} \hat{M}_a$ is the electron-phonon-photon coupling operator. 
In compact notation, the eigenvalue problem of the electronic Hamiltonian reads ${\cal H}|n\rangle = \varepsilon_n |n\rangle$, where $\varepsilon_n$ is the energy of band $n$ with eigenvector $|n\rangle$. The Matsubara Green's function can then be written in the band basis as
\begin{align}
    \langle n|\hat G (i\omega_\nu)|m\rangle = \delta_{nm} G_n= \frac{ \delta_{nm} }{ i\omega_\nu-\varepsilon_n}, 
\end{align}
where $\omega_\nu= (2\nu+1) k_B T$ stands for the fermionic Matsubara energy and $\nu$ is an integer. We use the standard Matsubara sums \cite{Mahan} for one, two and three propagators, given by
\begin{align}
    \frac{1}{\beta} \sum_\nu G_{m}(i \omega_\nu) =& f(\varepsilon_m) = f_m \label{eq.1GMatsSum} 
    \\
    \frac{1}{\beta} \sum_\nu G_{n}(i\omega_\nu + i\omega) G_{m}(i\omega_\nu) =& \frac{1}{\hbar} \frac{f_{mn}}{\omega + \omega_{mn}} \label{eq.2GMatsSum} 
    \\
    \frac{1}{\beta} \sum_\nu G_l(i\omega_\nu+i\omega_p) G_n(i\omega_\nu+i\omega_1) G_m(i\omega_\nu) =& \frac{1}{\hbar^2} \left\{  
    \frac{f_{mn}}{(\omega_1-\omega_{nm})(\omega_p-\omega_{lm})} + \frac{f_{ln}}{(\omega_2-\omega_{ln})(\omega_p-\omega_{lm})} \right\}
    , \label{eq.3GMatsSum}
\end{align}
where $\beta = 1/k_B T$ is the inverse temperature and $f_m$ denotes the Fermi–Dirac distribution for band $m$. We define $f_{mn} = f_n - f_m$, and $\omega_{nm} = (\varepsilon_n - \varepsilon_m)/\hbar$ is the energy difference between bands $n$ and $m$, expressed in frequency units.
With these sums, we compute the explicit values of each diagram, which are
\begin{align}
    \chi^{\rm A}_{abc} (\omega_p;\omega_1,\omega_2) =&-\frac{e^2}{2\hbar^2 (i\omega_1)(i\omega_2)}\sum_{\bf p} 
    \sum_{mnl} \bigg \{\frac{f_{mn} M^{ml}_a v^{ln}_c v^{nm}_b}{(\omega_1 + i\gamma-\omega_{nm})(\omega_p+i\Gamma-\omega_{lm})} + \frac{f_{mn} M^{lm}_a v^{mn}_c v^{nl}_b}{(\omega_2 + i\gamma-\omega_{mn})(\omega_p+i\Gamma-\omega_{ml})} 
    \nonumber\\&+ [b,\omega_1 \leftrightarrow c,\omega_2] \bigg \} 
    \label{eq:chi-A}
    \\
    \chi^{\rm B}_{abc} (\omega_p;\omega_1,\omega_2) =& \frac{-e^2}{2\hbar (i\omega_1)(i\omega_2)} \sum_{\bf p} \sum_{mn} \bigg\{\frac{f_{mn} M^{mn}_{ac} v^{nm}_b}{\omega_1 + i\gamma + \omega_{mn}} + [b,\omega_1 \leftrightarrow c,\omega_2] \bigg\}
    \label{eq:chi-B}
    \\
    \chi^{\rm C}_{abc} (\omega_p;\omega_1,\omega_2) =& \frac{-e^2}{2\hbar (i\omega_1)(i\omega_2)}\sum_{\bf p} \sum_{mn} \frac{f_{mn}M^{lm}_a v^{nm}_{bc}}{\omega_p+i\Gamma + \omega_{mn}}
    \label{eq:chi-C}
    \\
    \chi^{\rm D}_{abc} (\omega_p;\omega_1,\omega_2) =& -\frac{e^2}{2(i\omega_1)(i\omega_2)} \sum_{\bf p} \sum_m f_m M^{mm}_{abc} 
    \label{eq:chi-D}
\end{align}
where $O^{mn}=\langle m|\hat O|n\rangle$ is the matrix element of operator $\hat O$. 
Here, we include a small imaginary part in the frequency to account for phenomenological damping. Specifically, we add $\gamma$ to the frequencies $\omega_1$ and $\omega_2$, and $\Gamma$ to their sum, $\omega_p$. Physically, in the case of rectified Raman force we are interested in, $\gamma$ represents interband damping, while $\Gamma$ accounts for intraband damping \cite{Holder_TRS&QG}.
\section{Rectified Raman force function}
The rectified Raman force is obtained by setting $\omega_1 = -\omega_2 = \omega$, which implies $\omega_p = 0$. In general, the total rectified force can be decomposed into resonant and off-resonant contributions, where we show that the resonant part consists of both injection and shift terms, which are the main focus of this study. However, we also analyze the off-resonant term later. 
We additionally note here that the rectified force response to linearly-polarized (LP) and circularly-polarized (CP) light can be obtained by taking the real and imaginary parts of the response function, respectively \cite{rostami2022}.

\subsection{Injection force}
Upon taking the rectified case, the susceptibility term of Eq. \eqref{eq:chi-A} (Fig. \ref{fig:feyn}a) can be split into two parts, with $\chi^{\rm A}_{abc}(\omega)=\chi^{\rm inj}_{abc}(\omega)+\gamma^{\triangle}_{abc}(\omega)$. The first part is
\begin{align}
    \chi^{\rm inj}_{abc}(\omega)= 
    \frac{-e^2}{2\hbar {\omega}^2} \lim_{\omega_p\to0}\frac{1}{\omega_p+i\Gamma}\sum_{\bm{p}} \sum_{mn} \Bigg\{\frac{f_{mn} M^{mm}_a v^{mn}_c v^{nm}_b}{\omega + i\gamma-\omega_{nm}} + \frac{f_{mn} M^{mm}_a v^{mn}_c v^{nm}_b}{-\omega + i\gamma-\omega_{mn}} + [b,\omega \leftrightarrow c,-\omega] \Bigg\}, \label{eq.InitInj}
\end{align}
whose resonant component the injection force susceptibility. After some algebra, this can be simplified to give
\begin{align}
    \chi^{\rm inj}_{abc}(\omega)
    =
    \frac{-e^2}{2\hbar {\omega}^2 } \lim_{\omega_p\to0}\frac{1}{\omega_p+i\Gamma}\sum_{\bm{p}} \sum_{mn} \Bigg \{ \frac{f_{mn} (M^{mm}_a - M^{nn}_a) \omega_{nm}^2 Q_{bc}^{nm}}{\omega + i\gamma-\omega_{nm}} - \frac{f_{mn} (M^{mm}_a - M^{nn}_a) \omega_{nm}^2 Q_{bc}^{nm}}{\omega - i\gamma-\omega_{nm}} \Bigg \},\label{eq.InjPreCL}
\end{align}
where $Q_{bc}^{nm}$ is notably the band-resolved quantum geometric tensor which is given by 
\begin{align}
  Q_{bc}^{nm} = \frac{v^{nm}_b v_c^{mn}}{\omega_{nm}^2}=g_{bc}^{nm}-\frac{i}{2} \Omega_{bc}^{nm}  
\end{align}
in which $g_{bc}^{nm}$ and $\Omega_{bc}^{nm}$ are the band-resolved (interband) quantum metric and Berry curvature, respectively.
The second part, meanwhile, is 
\begin{align}
   \gamma^{\triangle}_{abc} (\omega) = \frac{-e^2}{2\hbar^2\omega^2} \sum_{\bm{p}} \sum_{mnl} \Bigg\{\frac{f_{mn} M^{ml}_a v^{ln}_c v^{nm}_b \eval_{l \neq m}}{(\omega + i\gamma-\omega_{nm})(i\Gamma-\omega_{lm})} + \frac{f_{mn} M^{lm}_a v^{mn}_c v^{nl}_b \eval_{l \neq m}}{(-\omega + i\gamma-\omega_{mn})(i\Gamma-\omega_{ml})}  + [b,\omega \leftrightarrow c,-\omega] \Bigg\}
\end{align}
where this term will be canceled out with a counter term emerging from the shift diagram in the clean limit. This delicate issue will be addressed in subsection \ref{app.cancel}.

Looking back at the first part, we now take the resonant ($\delta$-function) contribution of the clean limit ($\Gamma\to 0$ and $\gamma\to 0$), which can be separated from the off-resonant contribution using
\begin{align}
   \lim_{\gamma\to0} \frac{1}{\omega - \omega_{nm} + i\gamma} = \mathcal{P} \left( \frac{1}{\omega - \omega_{nm}} \right) - i\pi \delta(\omega - \omega_{nm}), \label{eq.cleanlim}
\end{align}
where $\mathcal{P}$ denotes the Cauchy principal value. This singular resonant part then leads to the injection force susceptibility through $\chi^{\rm inj ,\delta}_{abc}(\omega)=  \lim_{\omega_p \to 0}\alpha^{\rm inj}_{abc}(\omega)/i\omega_p$, with this injection force susceptibility given by
\begin{align}
    \alpha^{inj}_{abc}(\omega)
    =& -\frac{\pi e^2}{\hbar^2} \sum_{\bm{p}} \sum_{mn} f_{mn} \Delta_a^{mn} Q_{bc}^{nm} \delta(\omega -\omega_{nm}),
\end{align}
where $\Delta_a^{mn} = M^{mm}_a - M^{nn}_a$. In the main text, $\alpha^{inj}_{abc}(\omega)$ is described in relation to the total susceptibility in Eq. (3). This is a very simple form reminiscent of the injection current term written in terms of quantum geometry \cite{Ahn_prx_2020,Watanabe_prx_2021}. Splitting into LP and CP responses is then as simple as taking the real and imaginary components of $Q_{bc}^{nm}$. 
\subsection{Shift force}
As with Eq. \eqref{eq:chi-A}, we can rewrite the susceptibility contribution from Eq. \eqref{eq:chi-B} (Fig. \ref{fig:feyn}b) in two parts, as $\chi^{\rm B}_{abc}(\omega) = \chi^{\rm shi}_{abc}(\omega)+\gamma^{\rm O}_{abc} (\omega)$. Using the covariant derivative approach \cite{VenturaGaugeCov,Parker} with respect to phonon displacement in the $a$-direction,
\begin{align}
    M_{ab}^{mn} = \langle m|\hat M_{ab}|n\rangle =& \partial_{u_a} v_{b}^{mn} - i\comm{\hat{\mathbb{A}}_a}{\hat{v}_b}^{mn} = \partial_{u_a} v_{b}^{mn} -i \sum_l \big(\mathbb{A}_a^{ml} v_b^{ln} - v_b^{ml} \mathbb{A}_a^{ln} \big), \label{eq.PhononCovDev}
\end{align}
where the phononic Berry connection is defined as
\begin{align}
    \mathbb{A}^{mn}_a 
    = \langle m | \hat{\mathbb{A}}_a | n \rangle 
    = i \langle m | \partial_{u_a} | n \rangle,
\end{align}
we obtain the first part, whose resonant component gives the shift force susceptibility, as 
\begin{align}
    \chi^{\rm shi}_{abc}(\omega)=
    \frac{-e^2}{2\hbar \omega^2} \sum_{\bm{p}} \sum_{mn} f_{mn} \Bigg \{ \frac{\Big(\partial_{u_a} v_c^{mn} -i \big(\mathbb{A}_a^{mm} v_c^{mn} - v_c^{mn} \mathbb{A}_a^{nn} \big) \Big) v^{nm}_b}{\omega + i\gamma + \omega_{mn}} + [b,\omega \leftrightarrow c,-\omega] \Bigg\}\label{eq.InitShift}.
\end{align}
The second part, meanwhile, is given by
\begin{align}
    \gamma^{\rm O}_{abc}(\omega) = \frac{-e^2}{2\hbar\omega^2} \sum_{\bm{p}} \sum_{mnl} f_{mn}\Bigg\{ \frac{- i  \mathbb{A}_a^{ml} v_c^{ln} v^{nm}_b \eval_{l \neq m}}{\omega + i\gamma + \omega_{mn}} + \frac{-i \mathbb{A}_a^{lm} v_c^{nl} v^{mn}_b \eval_{l \neq m} )}{\omega + i\gamma - \omega_{mn}} + [b,\omega \leftrightarrow c,-\omega] \Bigg\},
\end{align}
which cancels $\gamma^{\triangle}_{abc}(\omega)$ in the clean limit, as discussed in the following subsection \ref{app.cancel}. 

Turning back to the first part, we represent velocity matrix elements in polar form, as $v_c^{mn} = \abs{v_c^{mn}} e^{-i \phi_c^{mn}}$ (noting that $\phi_{c}^{mn} = \Im \ln v_{c}^{mn} $),
which after some algebra gives us
\begin{align}
\chi^{\rm shi}_{abc}(\omega)=
     \frac{-e^2}{2\hbar \omega^2} \sum_{\bm{p}} \sum_{mn} f_{mn} \left \{ \frac{ \Big( \abs{v^{nm}_b} \partial_{u_a} \abs{v_c^{mn}} e^{-i (\phi_c^{mn} + \phi^{nm}_b)} -i \omega_{nm}^2 \mathbb{R}_{a;c}^{mn} Q_{bc}^{nm} \Big)}{\omega + i\gamma + \omega_{mn}} + [b,\omega \leftrightarrow c,-\omega] \right \} ,
\end{align}
where we can define the \textit{phononic shift vector} as
\begin{align}
    \mathbb{R}_{a;c}^{mn} = \partial_{u_a} \phi_{c}^{mn} + (\mathbb{A}_a^{mm} - \mathbb{A}_a^{nn}). \label{eq.PhSV}
\end{align}
Taking the resonant contribution in the clean limit, and following some basic algebra and use of the relation $ v_b^{mn} = i \omega_{mn} \mathcal{A}_b^{mn} $, which expresses the interband velocity matrix element in terms of the electronic Berry connection, $\mathcal{A}_b^{mn} = i\hbar \langle m | \partial_{p_b} | n \rangle $, we obtain the shift force susceptibility as
\begin{align}
    \beta^{\rm shi}_{abc}(\omega)
    = \frac{i\pi e^2}{2\hbar} \sum_{\bm{p}} \sum_{mn} f_{mn} \left\{\big( \abs{\mathcal{A}^{nm}_b} \partial_{u_a} \abs{\mathcal{A}_c^{nm}} - \abs{\mathcal{A}^{nm}_c} \partial_{u_a} \abs{\mathcal{A}_b^{nm}} \big) e^{-i (\phi^{nm}_b - \phi_c^{nm})} -i \big(\mathbb{R}_{a;c}^{mn} + \mathbb{R}_{a;b}^{mn} \big) Q_{bc}^{nm} \right\} \delta(\omega - \omega_{nm}).
\end{align}
This expression is rather complicated and opaque, and to make progress, we consider specific cases for the response to LP and CP light separately (in the way outlined above). For LP incoming light, we can, without loss of generality, assume that the input polarizations are identical, i.e., $c=b.$ In this case, the expression simplifies significantly to
\begin{align}
    \beta^{\mathrm{shi}-\mathrm{LP}}_{abb}(\omega)
    = \frac{\pi e^2}{\hbar} \sum_{\bm{p}} \sum_{mn} f_{mn} \mathbb{R}_{a;b}^{mn} \Re \left[Q_{bb}^{nm}\right] \delta(\omega - \omega_{nm}),
\end{align}
which resembles the well-known shift current formula expressed in terms of the quantum geometric tensor~\cite{Ahn_prx_2020, Watanabe_prx_2021}, whose real part corresponds to the quantum metric.

For CP light, we reformulate the expression using the chiral Berry connection and the chiral shift vector, as introduced in the context of the gyration (circular shift) current \cite{Watanabe_prx_2021}. The chiral Berry connections are defined as
\begin{align}
    \mathcal{A}_{\pm}^{mn} 
    = \frac{1}{\sqrt{2}} (\mathcal{A}_{b}^{mn} \pm i \mathcal{A}_{c}^{mn}) 
    = |\mathcal{A}_{\pm}^{mn}| e^{-i\phi_{\pm}^{mn}} 
    = [\mathcal{A}_{\mp}^{nm}]^*,
\end{align}
where the $\pm$ indices denote the two circular polarizations. The corresponding chiral phononic shift vector is given by
\begin{align}
    \mathbb{R}_{a;\pm}^{mn} 
    = \partial_{u_a} \phi_{\pm}^{mn} + (\mathbb{A}_a^{mm} - \mathbb{A}_a^{nn}), 
    \label{eq.ChiPhSV}
\end{align}
which captures the phase winding of the chiral Berry connection along with the difference in diagonal Berry connections.
Using these definitions, the shift force susceptibility to CP light becomes
\begin{align}
    \beta^{\mathrm{shi}-\mathrm{CP}}_{abc}(\omega)
    = \frac{\pi e^2}{2\hbar} \sum_{\bm{p}} \sum_{mn} f_{mn} 
    \left( |\mathcal{A}_{+}^{mn}|^2 \mathbb{R}_{a;+}^{mn} 
         - |\mathcal{A}_{-}^{mn}|^2 \mathbb{R}_{a;-}^{mn} 
    \right) 
    \delta(\omega - \omega_{nm}).
\end{align}
The squared chiral Berry amplitudes can be further expressed in terms of quantum geometric quantities as~\cite{Watanabe_prx_2021}
\begin{align}
    |\mathcal{A}_{\pm}^{mn}|^2 
    = \frac{g_{bb}^{mn} + g_{cc}^{mn} \mp \Omega_{bc}^{mn}}{2}.
\end{align}
Substituting this back into the previous expression yields
\begin{align}
    \beta^{\mathrm{shi}-\mathrm{CP}}_{abc}(\omega)
    = \frac{\pi e^2}{4\hbar} \sum_{\bm{p}} \sum_{mn} f_{mn} 
    \left\{ 
        (g_{bb}^{mn} + g_{cc}^{mn}) (\mathbb{R}_{a;+}^{mn} - \mathbb{R}_{a;-}^{mn}) 
        - \Omega_{bc}^{mn} (\mathbb{R}_{a;+}^{mn} + \mathbb{R}_{a;-}^{mn})
    \right\} 
    \delta(\omega - \omega_{nm}),
\end{align}
where we see contributions from both the symmetric (quantum metric) and antisymmetric (Berry curvature) parts of the quantum geometric tensor. This structure highlights the geometric origin of the Raman force response under circularly polarized excitation, which closely resembles that of the nonlinear photocurrent reported in Ref.~\cite{Watanabe_prx_2021}.
\subsection{Cancellation of counter terms from shift and injection diagrams}\label{app.cancel}
In the contributions from the injection and shift diagrams (Figs. \ref{fig:feyn}a, b), after removing the parts that contribute to the injection and shift force susceptibilities, we are left with:
\begin{align}
    \gamma^{\triangle}_{abc}(\omega) + \gamma^{\rm O}_{abc}(\omega)
    = \frac{-e^2}{2\hbar^2\omega^2} \sum_{\bm{p}} \sum_{mnl} f_{mn}\Bigg\{&\frac{ M^{ml}_a v^{ln}_c v^{nm}_b \eval_{l \neq m}}{(\omega + i\gamma-\omega_{nm})(i\Gamma-\omega_{lm})} + \frac{ M^{lm}_a v^{mn}_c v^{nl}_b \eval_{l \neq m}}{(-\omega + i\gamma-\omega_{mn})(i\Gamma-\omega_{ml})} 
    \nonumber \\
    +& \frac{- i \mathbb{A}_a^{ml} v_c^{ln} v^{nm}_b \eval_{l \neq m}}{\omega + i\gamma + \omega_{mn}} + \frac{-i \mathbb{A}_a^{lm} v_c^{nl} v^{mn}_b \eval_{l \neq m} )}{\omega + i\gamma - \omega_{mn}} + [b,\omega \leftrightarrow c,-\omega] \Bigg\}.
\end{align}
We treat the response in the intrinsic geometric limit, where impurity, disorder, and many-body scattering (dephasing) rates are negligible. The intrinsic response is obtained by first taking the clean limit, 
$\lim_{\{\Gamma,\gamma\} \to 0^+}$, at fixed band gap, and for the gapless case, the gap is sent to zero at the end: 
$\lim_{\text{gap} \to 0} \lim_{\{\Gamma,\gamma\} \to 0^+}$. 
This protocol captures the clean-system cancellation of the first and second lines in the above expression, independent of the magnitude of the band gap---that is, it remains valid even for an infinitesimal gap, as long as the gap exceeds the negligible scattering rates.  Therefore, in this limit, we can neglect the $\Gamma$ term and replace $i\Gamma - \omega_{lm} \to -\omega_{lm}$ in the denominators on the first line, yielding:
\begin{align}
    \gamma^{\triangle}_{abc}(\omega) + \gamma^{\rm O}_{abc}(\omega)
    = \frac{-e^2}{2\hbar^2\omega^2} \sum_{\bm{p}} \sum_{mnl} f_{mn}\Bigg\{& \frac{ M^{ml}_a v^{ln}_c v^{nm}_b \eval_{l \neq m}}{(\omega + i\gamma+\omega_{mn})(\omega_{ml})} + \frac{ M^{lm}_a v^{mn}_c v^{nl}_b \eval_{l \neq m}}{(-\omega + i\gamma-\omega_{mn})(\omega_{lm})} 
     \nonumber \\
    +& \frac{- i \mathbb{A}_a^{ml} v_c^{ln} v^{nm}_b \eval_{l \neq m}}{\omega + i\gamma + \omega_{mn}} + \frac{-i  \mathbb{A}_a^{lm} v_c^{nl} v^{mn}_b \eval_{l \neq m} }{\omega + i\gamma - \omega_{mn}} + [b,\omega \leftrightarrow c,-\omega] \Bigg\}.
\end{align}
Now, using the identity $M_a^{ml} = i \varepsilon_{ml} \mathbb{A}_a^{ml}$ for $m \neq l$ in the second line, and then simplifying and explicitly showing all terms, we get
\begin{align}
    \gamma^{\triangle}_{abc}(\omega) + \gamma^{\rm O}_{abc}(\omega)  
    =& \frac{e^2}{2\hbar^2\omega^2} \sum_{\bm{p}} \sum_{mnl} \frac{f_{mn}}{\omega_{lm}} \Bigg\{ \frac{M^{ml}_a v^{ln}_c v^{nm}_b}{\omega + i\gamma+\omega_{mn}} - \frac{M^{lm}_a v^{mn}_b v^{nl}_c}{\omega + i\gamma-\omega_{mn}} + \frac{M^{ml}_a v^{ln}_b v^{nm}_c}{-\omega + i\gamma+\omega_{mn}} - \frac{M^{lm}_a v^{mn}_c v^{nl}_b }{-\omega + i\gamma-\omega_{mn}}  
    \nonumber \\
    &\hspace{2.4cm}- \frac{M_a^{ml} v_c^{ln} v^{nm}_b}{\omega + i\gamma + \omega_{mn}} + \frac{M_a^{lm} v_c^{nl} v^{mn}_b}{\omega + i\gamma - \omega_{mn}} - \frac{M_a^{ml} v_b^{ln} v^{nm}_c}{-\omega + i\gamma + \omega_{mn}} + \frac{M_a^{lm} v_b^{nl} v^{mn}_c}{-\omega + i\gamma - \omega_{mn}} \Bigg\}\eval_{l \neq m},
\end{align}
and thus in the clean limit we obtain an identically exact cancellation as follows 
\begin{align}
      \gamma^{\triangle}_{abc}(\omega) + \gamma^{\rm O}_{abc}(\omega) = 0,
\end{align}
as the terms on the top row clearly each cancel with the term directly below it. This reasoning can be compared to the cancellation of the counter terms for the injection and shift photocurrents, following a similar logic to that used in Sec.~III~D of Ref.~\cite{Watanabe_prx_2021}, for example.

\subsection{Off-resonant force}
Here we examine both parts of the off-resonant Raman force, which are not treated in the main text.  The first part arises from taking the principal value terms in the clean limit, Eq. \eqref{eq.cleanlim}, instead of the Dirac delta (which gives the injection and shift forces). The second part originates from the other two susceptibility terms given by Eqs.~\eqref{eq:chi-C} and \eqref{eq:chi-D}, represented by the oval diagrams in Fig.~\ref{fig:feyn}c and d. We show that, other than for a nonlinear Drude term, one can write these responses in terms of the quantum geometric tensor, just like the resonant components.

\subsubsection{Off-Resonant contribution from diagrams (a) and (b): ${\beta}^{\rm off,1}_{abc}$}
We begin with the off-resonant component of the triangle diagram in Fig.~\ref{fig:feyn}a, which also describes the resonant displacive (injection) Raman force. Taking the principal value part of the clean limit of Eq.~\eqref{eq.InjPreCL} yields
\begin{align}
    \alpha^{\rm off}_{abc}(\omega)
    =& \frac{-e^2}{2\hbar^2 \omega^2} \sum_{\bm{p}} \sum_{mn} f_{mn}\pv\Bigg \{\frac{ (M^{mm}_a - M^{nn}_a) \omega_{nm}^2 Q_{bc}^{nm}}{\omega - \omega_{nm}} - \frac{ (M^{mm}_a - M^{nn}_a) \omega_{nm}^2 Q_{bc}^{nm}}{\omega - \omega_{nm}} \Bigg\} = 0,
\end{align}
indicating the absence of an off-resonant counterpart to the injection force. This implies both that the off-resonant susceptibility is completely impulsive in nature, and the displacive susceptibility comes purely from resonant interband transitions.

Next, we consider the off-resonant component of the oval diagram in Fig.~\ref{fig:feyn}b, which serves as the off-resonant analogue to the shift force. Taking the principal value part of the clean limit of Eq.~\eqref{eq.InitShift} yields
\begin{align}
    {\beta}^{\rm off,1}_{abc}(\omega)
    = \frac{-e^2}{2\hbar \omega^2} \sum_{\bm{p}} \sum_{mn} f_{mn}\pv\Bigg \{\frac{v^{nm}_b \partial_{u_a} v_c^{mn} -i \big(\mathbb{A}_a^{mm} - \mathbb{A}_a^{nn} \big) v^{nm}_b v_c^{mn} }{\omega - \omega_{nm}} + [b,\omega \leftrightarrow c,-\omega] \Bigg\}.
\end{align}
Writing explicitly the second term and exchanging $m \leftrightarrow n$ in this term yields, after some algebra, an expression in terms of the quantum geometric tensor $Q_{bc}^{nm}$:
\begin{align}
    {\beta}^{\rm off,1}_{abc}(\omega)
    = \frac{-e^2}{2\hbar^2 \omega^2} \sum_{\bm{p}} \sum_{mn} f_{mn} \pv\Bigg \{\frac{2 \omega_{nm} \Delta_a^{nm} Q_{bc}^{nm} + \hbar\omega_{nm}^2 \partial_{u_a} Q_{bc}^{nm}}{\omega - \omega_{nm}} \Bigg\}, \label{eq.PVSusc}
\end{align}
where we use that EPC-difference, $\Delta_a^{nm} = \hbar\partial_{u_a} \omega_{nm}$. In the second term, it enters via a displacement derivative, $\partial_{u_a} Q^{mn}_{bc}$: the phononic counterpart to the momentum-derivatives of $Q^{mn}_{bc}$ that define quantum geometric \emph{dipoles} in the photogalvanic effect \cite{Watanabe_prx_2021,Anyuan2023}. For LP and CP responses, we respectively call these the phononic dipoles of quantum metric and Berry curvature.

\subsubsection{Off-Resonant contribution from diagrams (c) and (d): ${\beta}^{\rm off,2}_{abc}$}
Here we analyze the two oval diagrams in Fig.~\ref{fig:feyn}c, d, corresponding to the terms given in Eqs.~\eqref{eq:chi-C} and \eqref{eq:chi-D}, which contribute to the susceptibility as
\begin{align}
    {\chi}^{\rm C}_{abc}(\omega) +{\chi}^{\rm D}_{abc}(\omega)=& \frac{-e^2}{2\omega^2} \sum_{\bm{p}} \Bigg \{ \sum_m f_m M^{mm}_{a;bc} + \sum_{mn} \frac{f_{mn} M^{mn}_a v^{nm}_{bc}}{i\hbar\Gamma - \varepsilon_{nm}} \Bigg \}.
\end{align}
Using the covariant derivative from Eq.~\eqref{eq.PhononCovDev} in the first term, expressing $M_a^{mn} = i \varepsilon_{nm} \mathbb{A}_a^{mn}$ and following some algebra, we rewrite the expression as
\begin{align}
    {\chi}^{\rm C}_{abc}(\omega) +{\chi}^{\rm D}_{abc}(\omega)
    =& \frac{-e^2}{2\omega^2} \sum_{\bm{p}} \Bigg \{ \sum_m f_m \partial_{u_a} v_{bc}^{mm} + \sum_{mn} f_{mn}\bigg[\frac{  M_a^{mn} v_{bc}^{nm}}{\varepsilon_{nm}}  + \frac{ M^{mn}_a v^{nm}_{bc}}{i\hbar\Gamma - \varepsilon_{nm}} \bigg] \Bigg\}.
\end{align}
Assuming a clean system far from band-touching (so that $i\hbar\Gamma$ can be neglected), the last two terms cancel, leaving
\begin{align}
    {\beta}^{\rm off,2}_{abc}(\omega) = 
     {\chi}^{\rm C}_{abc}(\omega) +{\chi}^{\rm D}_{abc}(\omega)=& \frac{-e^2}{2\omega^2} \sum_{\bm{p}} \sum_m f_m \partial_{u_a} v_{bc}^{mm}.
\end{align}
Expanding this using the symmetrized (in $p_b$ and $p_c$) momentum covariant derivative \cite{VenturaGaugeCov}, and substituting $\partial_{u_a} v_b^{mm} = \partial_{p_b} M_a^{mm}$ and $v_c^{mn} = -i \omega_{nm} \mathcal{A}_c^{mn}$, we obtain
\begin{align}
    {\beta}^{\rm off,2}_{abc}(\omega)
    = \frac{-e^2}{2\omega^2} \sum_{\bm{p}} \Bigg \{ \sum_m f_m \partial_{p_b} \partial_{p_c} M_{a}^{mm} + \frac{1}{2} \sum_{mn} f_{mn} \partial_{u_a} \bigg(\frac{v_b^{mn} v_{c}^{nm} + v_c^{mn} v_{b}^{nm}}{\omega_{nm}} \bigg) \Bigg \}.
\end{align}
In the first term, the $p$-derivatives can be moved onto $f_m$, while the quantum metric appears in the second, giving
\begin{align}
    {\beta}^{\rm off,2}_{abc}(\omega)
    = \frac{-e^2}{2\omega^2} \sum_{\bm{p}} \bigg \{\sum_m \big(\partial_{p_b} \partial_{p_c} f_m \big) M_{a}^{mm} - \sum_{mn} f_{mn} \Big(\frac{\Delta_a^{mn}}{\hbar} g_{bc}^{mn} + \omega_{mn} \partial_{u_a} g_{bc}^{mn} \Big) \bigg\}. \label{eq.IntraSusc}
\end{align}
The first term resembles a higher-order Drude response, which describes the Drude DC photocurrent if the electron-phonon coupling operator is replaced by the velocity operator (i.e., $\hat{M}_a \to \hat{v}_a$), and shows the usual divergence for $\omega\to0$ \cite{Watanabe_prx_2021}.  
The second term, meanwhile, includes the phononic dipole of quantum metric similar to that in Eq.~\eqref{eq.PVSusc}.
Since this expression is fully real, it contributes only to the response under LP light.

As an example, Fig.~\ref{fig:SM_OffRes}a, b shows the LP and CP components of ${\beta}^{\mathrm{off},1}_{abc}(\omega)$ in the bilayer Haldane model. To highlight their high-frequency behavior, we omit the prefactor $(\hbar\omega)^{-2}$. Notably, the interband transition features differ significantly from their resonant counterparts, even though the spectral features occur at the same frequencies. On the other hand, the example spectra for the LP and CP components of ${\beta}^{\mathrm{off},2}_{abc}(\omega)$ are shown in Fig.~\ref{fig:SM_OffRes}c, d. The LP component exhibits a rapid decay with frequency, consistent with the expected $1/\omega^2$ scaling. The CP component vanishes, as predicted by Eq.~\eqref{eq.IntraSusc}, despite the presence of a nonzero Haldane gap ($\delta_H$), sublattice gap ($\delta$), and a source–drain current induced by a $\mathcal{C}_3$-symmetry-breaking momentum shift $\delta k_\nu$.

\begin{figure}[ht]
    \centering
\includegraphics[width=0.8\linewidth]{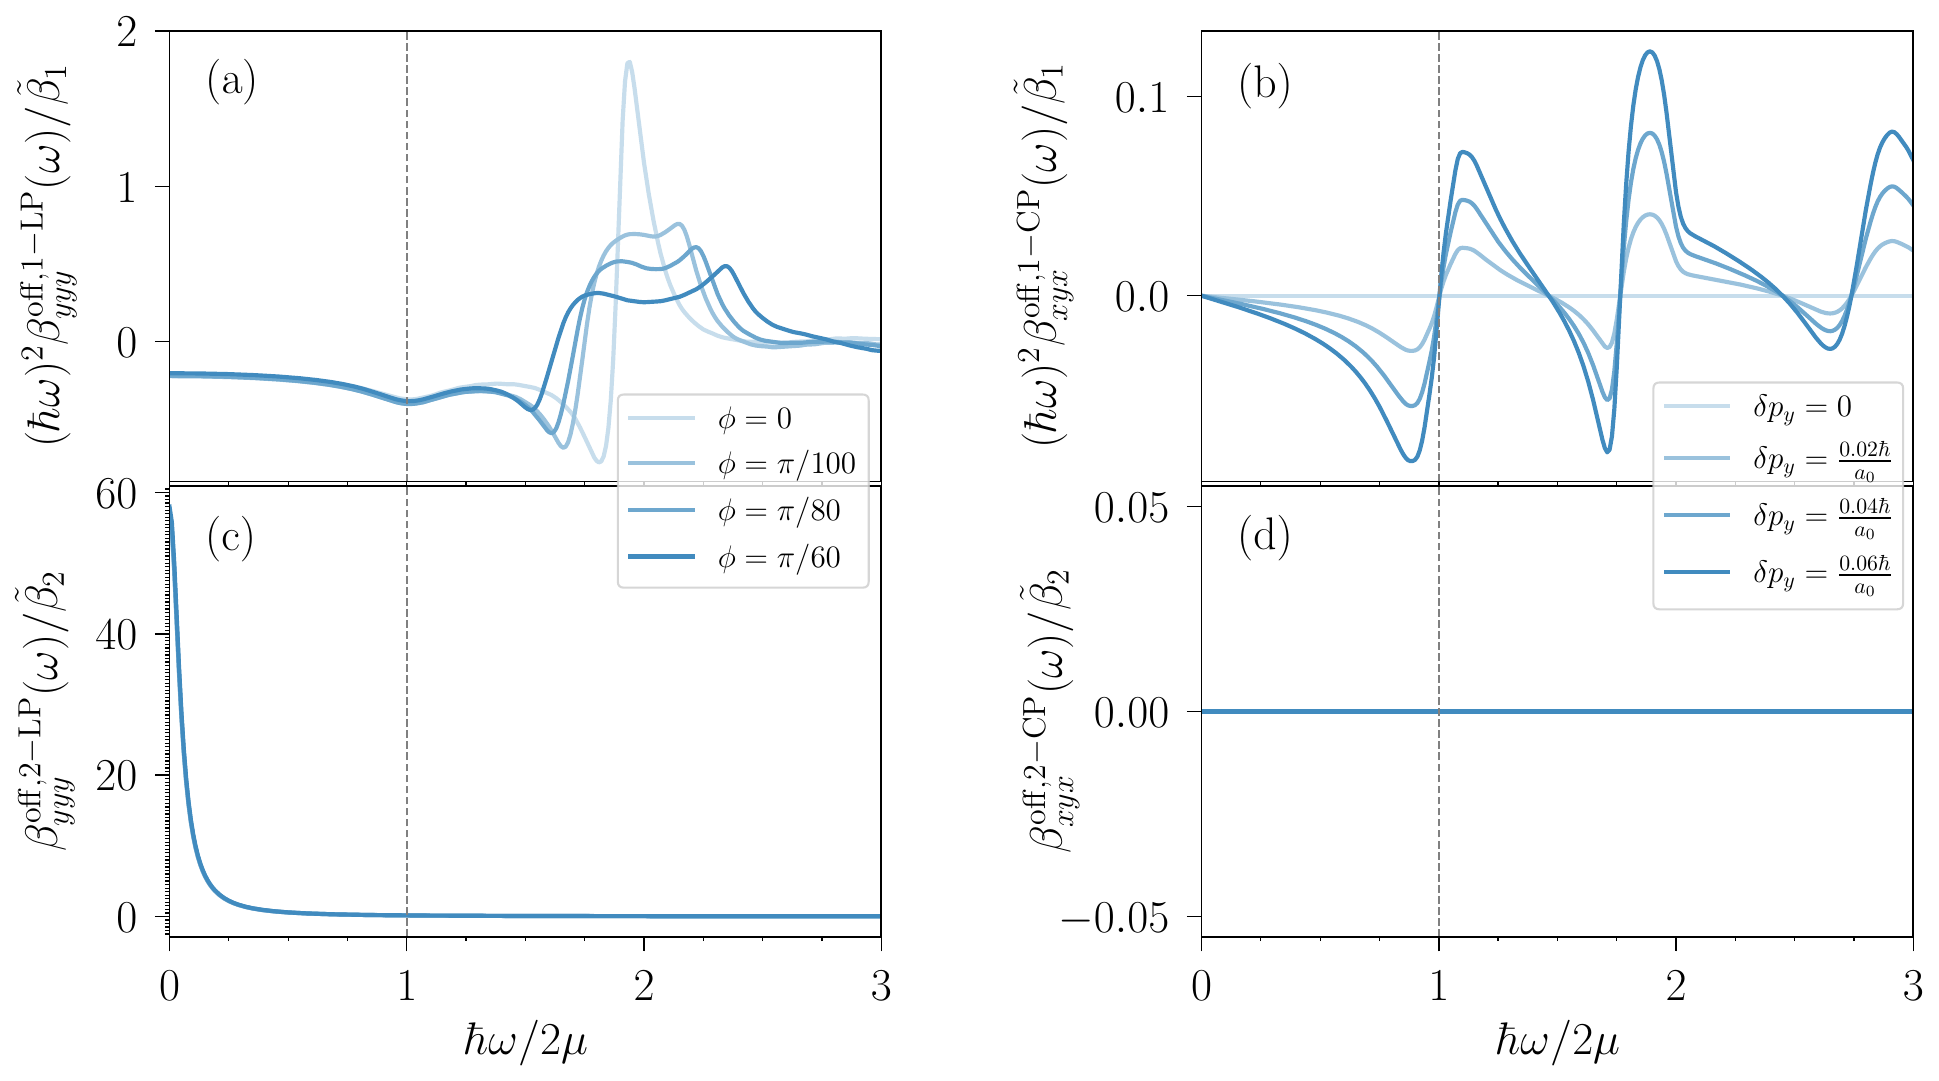}
    \caption {Spectra for the (a) LP and (b) CP component of off-resonant shear Raman force contribution ${\beta}^{\rm off,1}_{abc}(\omega)$ (Eq.~\ref{eq.PVSusc}) multiplied by $(\hbar\omega)^2$, and (c) the LP and (d) CP component of ${\beta}^{\rm off,2}_{abc}(\omega)$ (Eq.~\ref{eq.IntraSusc}) in the bilayer Haldane model. LP components (a) and (c) were obtained by varying Haldane phase, $\phi$ with sublattice gap, $\delta=0$ eV; CP components (b) and (d) varying $\delta p_y$: the electron momentum-shift due to a $y$-directional source-drain current flow, and with $\delta=0.05$ eV. In (c), we avoid the divergence at $\omega\to0$ by adding a small scattering rate of $0.01$ eV$/\hbar$ to $\omega$. In (d), we use finite values of $\phi=\pi/80$ and $\delta p_x = 0.03 \hbar a_0^{-1}$ to maximize symmetry-breaking. Note that  $\tilde\beta_1 = 0.5\, \mathrm{(eV)}^2 (\mathrm{nN}/\mathrm{V}^2)$ and $\tilde\beta_2 = 0.5\, (\mathrm{nN}/\mathrm{V}^2)$.}
    \label{fig:SM_OffRes}
\end{figure}

\section{Numerically-Accessible Phononic Shift Vector}
Here, we discuss how we obtain the phononic shift vector given by Eq. \eqref{eq.PhSV} in our numerical computation. It is difficult to evaluate directly due to the derivative with respect to phonon displacement, so we find an alternative form. We note that this method is easily transferable to compute the usual shift vector describing the shift photocurrent.
We start with the numerically-accessible term $M_{ab}^{mn} v_b^{nm}$, which upon expansion with the phononic covariant derivative of Eq. \eqref{eq.PhononCovDev} gives us, after use of the polar form for $v_b^{nm}$ and some algebra, that
\begin{align}
    M_{ab}^{mn} v_b^{nm} 
    =& (\partial_{u_a} \abs{v_{b}^{mn}}) \abs{v_b^{nm}} e^{-i(\phi_{b}^{mn} + \phi_{b}^{nm})} -i (\partial_{u_a} \phi_{b}^{mn}) v_{b}^{mn} v_b^{nm} - i v_{b}^{mn} v_b^{nm} (\mathbb{A}_a^{mm}  - \mathbb{A}_a^{nn}) 
   \nonumber\\ 
    -& i\sum_l \left\{\mathbb{A}_a^{ml} v_{b}^{ln} \Big|_{l \neq m} - \mathbb{A}_a^{ln} v_{b}^{ml} \Big|_{l \neq n}\right\} v_b^{nm},
\end{align}
where the phases (which are antisymmetric in $n$ and $m$) cancel in the first term, and we see the phononic shift vector as defined in Eq. \eqref{eq.PhSV} appear between the second and third terms. Hence, we have
\begin{align}
    M_{ab}^{mn} v_b^{nm} =& \abs{v_b^{nm}}\partial_{u_a} \abs{v_{b}^{mn}}  -i \abs{v_{b}^{mn}}^2 \mathbb{R}_{a;b}^{mn} - i\sum_l \left\{\mathbb{A}_a^{ml} v_{b}^{ln} \Big|_{l \neq m} - \mathbb{A}_a^{ln} v_{b}^{ml} \Big|_{l \neq n}\right \} v_b^{nm}.
\end{align}
As the first term is fully real, the second is fully imaginary, while the third is, in general, complex, we can take just the imaginary part of both sides to get
\begin{align}
   \Im( M_{ab}^{mn} v_b^{nm}) =& - \abs{v_{b}^{mn}}^2 \mathbb{R}_{a;b}^{mn} - \Im\bigg\{i\sum_l (\mathbb{A}_a^{ml} v_{b}^{ln} \eval_{l \neq m} - \mathbb{A}_a^{ln} v_{b}^{ml} \eval_{l \neq n}) v_b^{nm}\bigg\}.
\end{align}
In the second term on the right-hand side, we can use $M_a^{mn} = i \varepsilon_{mn} \mathbb{A}_a^{mn}$ for $m \neq n$ to eliminate the non-Abelian phononic Berry connection.
Then, by simple rearrangement, we finally obtain the shift vector as
\begin{align}
    \mathbb{R}_{a;b}^{mn} =& - \frac{\Im( M_{ab}^{mn} v_b^{nm}) + \Im \sum_l \bigg \{\frac{M_a^{ml} v_{b}^{ln} v_b^{nm}}{\varepsilon_{ml}} \eval_{l \neq m} - \frac{M_a^{ln} v_{b}^{ml} v_b^{nm}}{\varepsilon_{ln}} \eval_{l \neq n} \bigg \} }{\abs{v_{b}^{mn}}^2},
\end{align}
which is easily calculable numerically.
We can perform similar analysis to obtain the chiral phononic shift vector of Eq. \eqref{eq.ChiPhSV} in a numerically-easily accessible form, which leads to
\begin{align}
     \mathbb{R}_{a;\pm}^{mn} =& - \frac{\Im(M_{a;\pm}^{mn} v_\mp^{nm}) + \Im \sum_l \bigg\{\frac{M_a^{ml} v_{\pm}^{ln} v_\mp^{nm}}{\varepsilon_{ml}} \eval_{l\neq m} - \frac{M_a^{ln}v_{\pm}^{ml} v_\mp^{nm}}{\varepsilon_{ln}} \eval_{l\neq n}\bigg\}}{\abs{v_{\pm}^{mn}}^2}.
\end{align}
Both the linear and chiral phononic shift vector expressions can be simplified further by canceling a factor of $v_b^{nm}$ and $v_{\mp}^{nm}$, respectively. The two can then written in a unified form, given by
\begin{align}
    \mathbb{R}_{a;\ell}^{mn} =& -{\rm Im} \left\{\frac{M_{a\ell}^{mn}}{v_\ell^{mn}} + \sum_{l \neq m} \frac{M_a^{ml} v_{\ell}^{ln}}{\varepsilon_{ml} v_{\ell}^{mn}} - \sum_{l \neq n} \frac{M_a^{ln} v_{\ell}^{ml} }{\varepsilon_{ln} v_{\ell}^{mn}} \right\},
\end{align}
with $\ell \rightarrow b$ for the linear and $\ell \rightarrow \pm$ for the chiral case, as written in Eq.~(6) in the main text. This expression can be simplified for the low-energy two-band system which we use later in the main text, where sums over bands $l$ each give only one term, and where $\hat{M}_a$ has no $p$-dependence. In this case, we get
\begin{align}
    \mathbb{R}_{a;\ell}^{mn,\text {2-band}} =& {\rm Im} \left\{ \frac{M_a^{mn} (v_{\ell}^{mm}-v_{\ell}^{nn})}{\varepsilon_{mn} v_{\ell}^{mn}} \right\}.
\end{align}
\section{Numerical result for CP injection and shift force}

\begin{figure}[b]
    \centering    \includegraphics[width=0.8\linewidth]{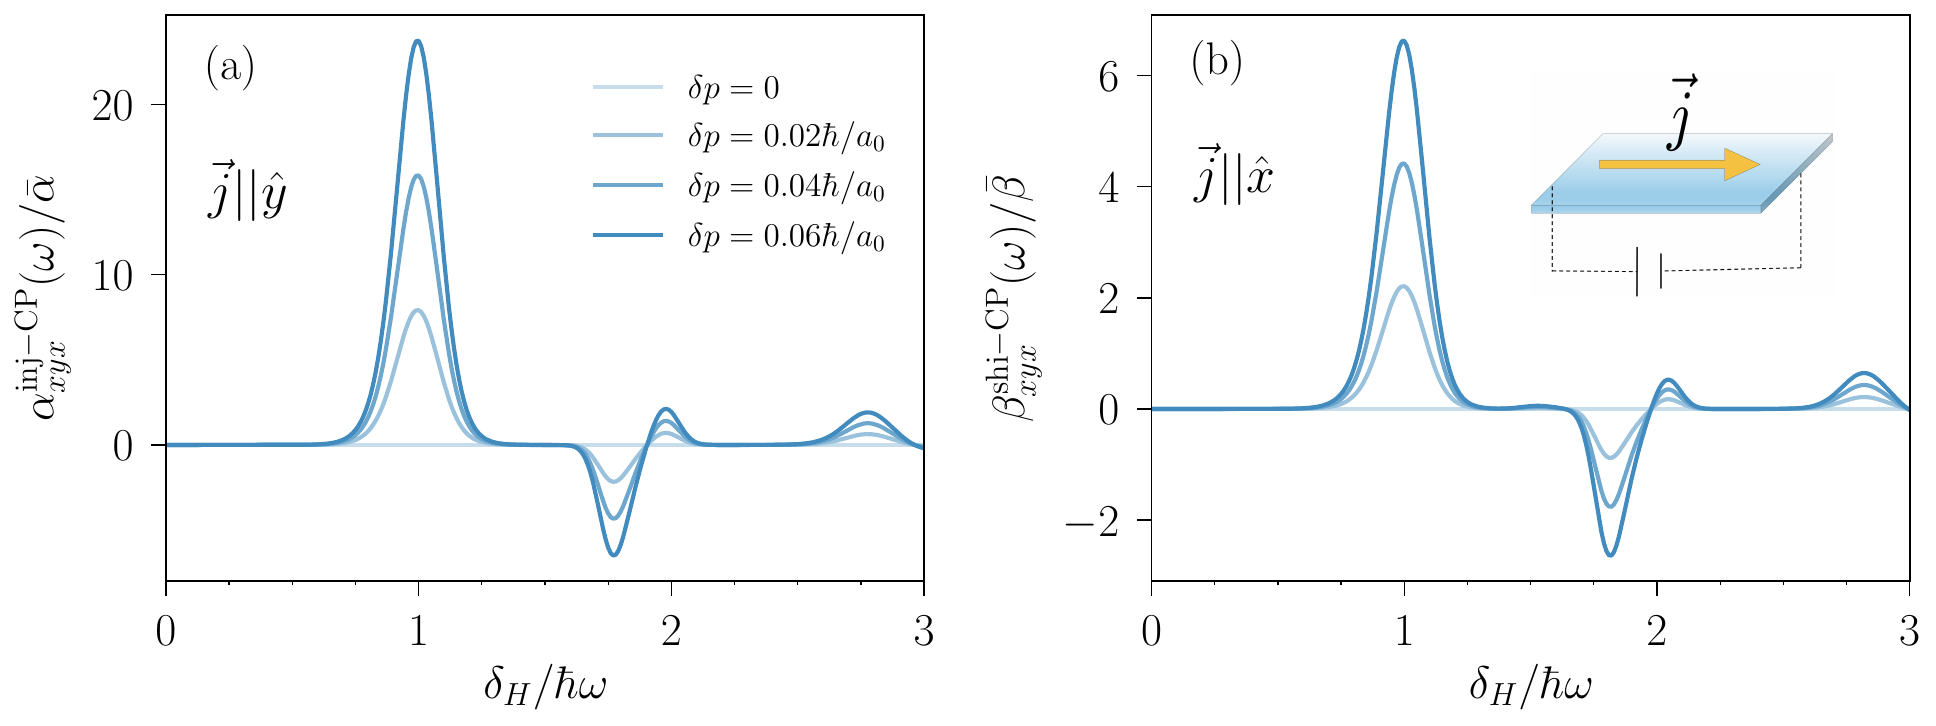}
    \caption{Spectra for CP (a) injection (b) shift shear Raman force susceptibility in the bilayer Haldane model. We obtain results for different source-sink current flows, $\vec{j}$, which generate a parallel shift, $\delta \bf{p}$ in electron momenta (which perturbs the Fermi distribution function), with the direction of the current and momentum shift being (a) $y$-directional and (b) $x$-directional. We set a temperature of 50 K, and (a) $\phi=0$ and $\delta=0.05$ eV, and (b) $\phi=\pi/80$ and $\delta=0.05$ eV. Note that $\bar\alpha = 50\, \mathrm{nN}/(\mathrm{V}^2 \, \mathrm{ps})$ and $\bar\beta = 0.5\, \mathrm{nN}/\mathrm{V}^2$, the same units used for the LP counterparts in Fig. 3 in the main text. The same values for parameters are used as for the LP resonant susceptibilities, as listed at the end of the caption of Fig. 3 in the main text.
    }
    \label{fig:SM_CPComps}
\end{figure}

Here, we briefly present and discuss the numerical results for the components of the resonant Raman shear force susceptibilities under circularly polarized (CP) light, plotted as a function of $\omega$ in the bilayer Haldane model. These correspond to the CP injection force and CP shift force responses, respectively described by Eqs.~(7) and (8) in the main text.

In the bilayer Haldane model, the presence of $\mathcal{C}_3$ symmetry forbids these CP resonant responses, even when they are allowed by $\mathcal{T}$- and $\mathcal{PT}$-symmetry (see Table~I in the main text). We therefore introduce an additional perturbation to break this symmetry---in our case, a unidirectional source-drain DC current flow as shown in the inset of Fig.~\ref{fig:SM_CPComps}b (although uniaxial strain could also serve as an alternative approach to break the rotational symmetry).
In the steady state, the DC current induces a rigid shift of the Fermi surface, characterized by the drift velocity. Using Boltzmann theory \cite{MooreCurrentInd2ndHar}, one can show that this current leads to a correction in the Fermi distribution function, given by $\delta f_m = \delta \bm{p} \cdot \nabla_{\bm{p}} f_m$, where the momentum shift is $\delta \bm{p} = e \tau \bm{E}_{\rm dc}$, and $\tau$ denotes the intraband relaxation time of the electrons. Fig.~\ref{fig:SM_CPComps} shows the CP (a) injection and (b) shift shear force susceptibilities at different momentum shift (i.e., DC currents). At zero $\delta p$, both CP responses vanish, as expected, while the finite current flow then induces nonvanishing susceptibilities, which increase with the magnitude of the current. 

Three distinct features are seen in the spectra for both CP injection and shift shear forces in Fig.~\ref{fig:SM_CPComps}, which are, from left to right: a peak at $\hbar\omega = 2\mu$ corresponding to the UVB-to-LCB transition, a peak derivative-like feature associated with the LCB-to-UCB transition, and a shallow peak from the LVB-to-LCB transition.
This current-induced shear force is driven by the current-induced stationary population distortion, \mbox{$\delta f_m$}, which is significant only near the Fermi surface. 
Considering a chemical potential (hence Fermi surface) in the LCB, and noting that all listed transitions involve the LCB, the fact that all three features exhibit sharp, peak-like behavior clearly originates from the fact that only electronic transitions in the vicinity of the Fermi surface can contribute to the CP Raman force responses, as only here does the necessary symmetry-breaking effect of the current flow make significant impact. The fact that the LCB-to-UCB feature has a shape different from that of the other two matches the case for the equivalent LP responses (in Fig. 3c, d in the main text), which in turn originates from the response being between two (nearly parallel) conduction bands, rather than one valence and one conduction band, as with the other two features.
\bibliography{refs}
\end{document}
